# Supplementary material for: Bundling dynamics regulates the active mechanics and transport in carbon nanotube networks
Source: arXiv:1108.2062 source file (2011-08-09)
Supplement: Supplementary file 1 [file SI.pdf]

# Supplementary Information for

## *Bundling dynamics regulates the electro-/thermo-mechanical coupling in aligned carbon nanotube networks*

Myung Gwan Hahm[*†], Hailong Wang[‡], Hyun Young Jung[*], Sanghyun Hong[*], Sung-Goo Lee[§], Sung-Ryong Kim[⊥], Moneesh Upmanyu[‡] and Yung Joon Jung[*]

[*]Department of Mechanical and Industrial Engineering, Northeastern University, Boston, Masschusetts, 02115, [†]Department of Mechanical Engineering and Materials Science, Rice University, Houston, Texas, 77005 USA, [‡]Group for Simulation and Theory of Atomic-Scale Material Phenomena (*st*AMP), Department of Mechanical and Industrial Engineering, Northeastern University, Boston, Masschusetts, 02115, [§]Information and Electronics Polymer Research Center, Korea Research Institute of Chemical Technology, Deajeon 305-600, Republic of Korea, [⊥]Department of Polymer Science and Engineering, Chungju National University, Chungbuk 380-702, Republic of Korea

Phone: (617) 373-3186, Fax: (617) 373-2921, E-mail: mupmanyu@neu.edu, jungy@coe.neu.edu

The supplementary text includes:

Figure S1

Figure S2

Figure S3

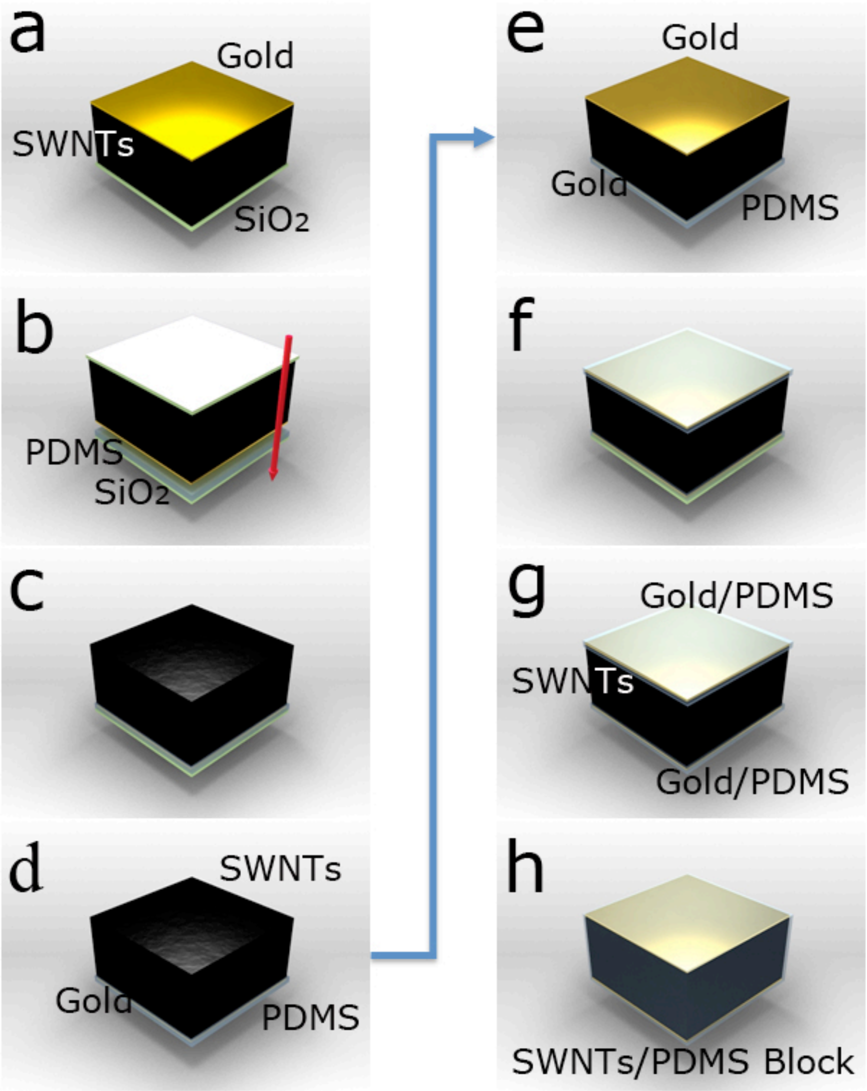


**Figure S1. Schematic illustration of the fabrication of S/CNN/S superstructure:** (a) Deposition of Ti (5 nm)/Au (150 nm) on as-grown vertically aligned SWNTs, (b) deposition of of 80% cured PDMS thin film (300 μm in thickness) on the top-side of the Ti/Au-coated SWNTs, (c) removal of $SiO_2$ wafer for after complete curing of PDMS thin film, (d) detachment of the $SiO_2$ wafer for PDMS thin film coating, (e) deposition of the second Ti/Au contact pad on the bottom-side of the superstructure after contact transfer, (f) deposition of the 80% cured PDMS on the second metal pad, (g), removal of the $SiO_2$ wafer from the bottom-side, and (h) finally PDMS infiltration and curing. A subset of the S/CNN/S structures are synthesized without removal of the $SiO_2$ wafers to facilitate stretching of the CNNs.

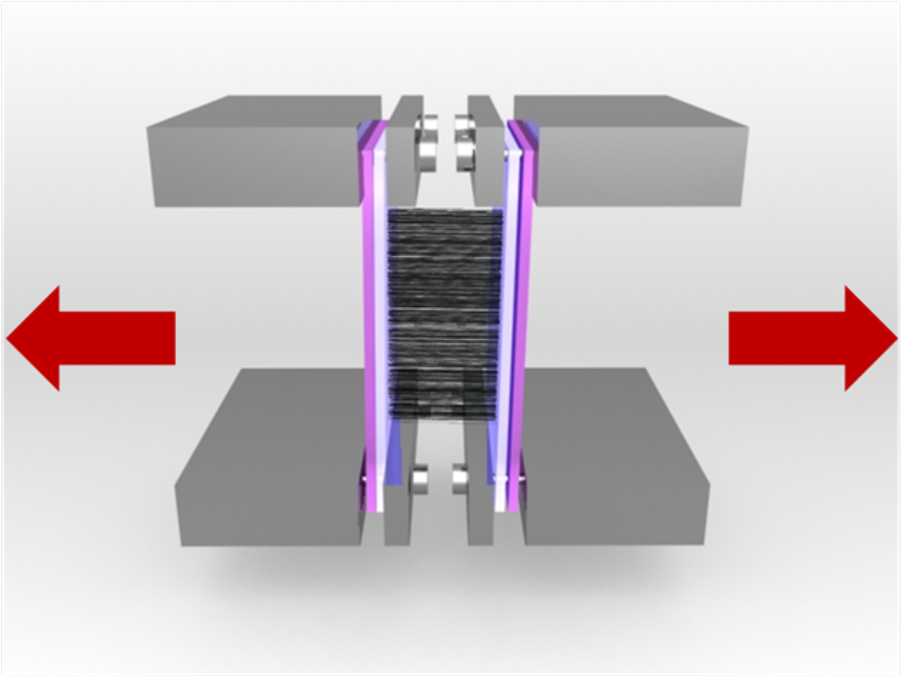

**Figure S2. Schematic illustration of the straining apparatus used stretch the S/CNN/S superstructure**. Flat plates that are clamped onto the silica layers and then pulled apart in a controlled fashion, indicated by the arrows.

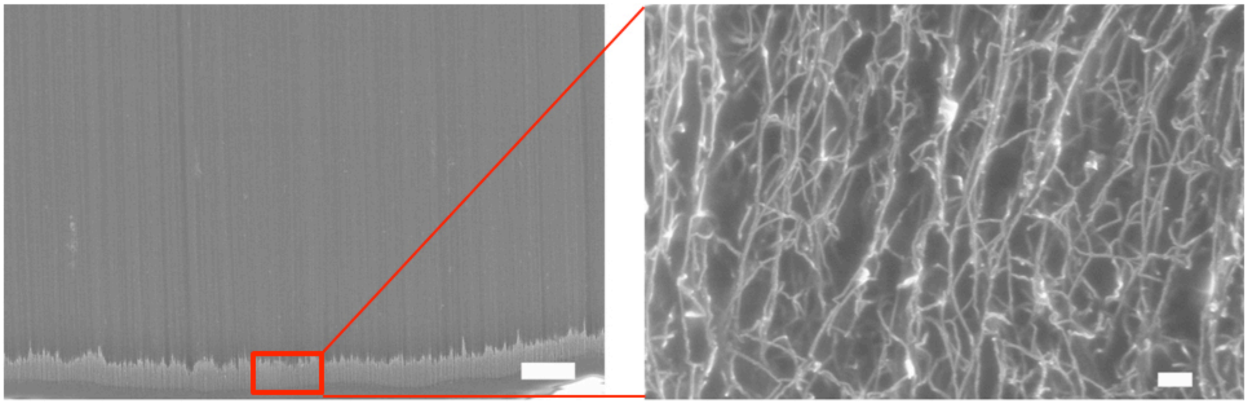

**Figure S3. Detailed characterization of the PDMS/SWNTs interfaces within the S/CNN/S superstructures**. (left) Low-magnification SEM image of bottom side of superstructure. The scale bar is 200 µm. (right) High-resolution of the interface region, showing SWCNTs which are anchored into the PDMS matrix. The scale bar is 200 nm.
